# Supplementary material for: A Survey of Multimodal Large Language Model from A Data-centric Perspective
Source: arXiv:2405.16640 source file (2024-07-18)
Supplement: Supplementary file 1 [file appendix.tex]

\section{appendix}

% \subsection{Data sources}

\subsection{Commonly Used X-Text Datasets}\label{sec:appen:datasets}
X-Test datasets are the most commonly used evaluation datasets. Here, we summarize Image-Text, Video-Text, Audio-Text and 3d-Text datasets.
\subsubsection{Image-Caption Datasets}\label{sec:appen:datasets:image-cap}
In this subsubsection, we provide a comprehensive summary of image caption datasets to help people find the most suitable datasets for MLLMs training.
\paragraph{General Image-Caption Datasets.} General image-caption datasets are datasets that contains image with short caption. Usually these captions are only one sentence or several words, describing the key character of the image.
\begin{itemize}
    \item \href{https://laion.ai/projects/}{\textbf{LAION-400M}}~\cite{schuhmann2021laion}. LAION-400M is a pioneering dataset for multimodal language-vision model training, comprising CLIP-filtered 400 million image-text pairs sourced from the Common Crawl web archive. These pairs are accompanied by CLIP embeddings and k-Nearest Neighbors (kNN) indices for efficient similarity searches. The dataset was processed through distributed parsing of Common Crawl's WAT files, extracting images with alt-texts as captions. Images and captions were then filtered based on character length, image size, and cosine similarity of CLIP embeddings to ensure relevance and quality. Additionally, duplicates were removed, and illegal contents were filtered out using CLIP embeddings. Less than 1\% of the images were tagged as Not Safe For Work (NSFW), allowing for easy exclusion. LAION-400M enables the broad research community to train and research large-scale multimodal models, previously limited to proprietary datasets. This dataset signifies a crucial step towards democratizing research in multimodal machine learning by providing a vast, diverse, and accessible resource for developing advanced language-vision models.
    
    \item \href{https://laion.ai/blog/laion-5b/}{\textbf{LAION-5B}}~\cite{schuhmann2022laion}. LAION-5B is the largest public image-text dataset to date, comprising over 5.8 billion examples derived from the Common Crawl web archive. It includes 2.32 billion English image-text pairs, 2.26 billion pairs in over 100 other languages, and 1.27 billion samples where a language couldn't be clearly identified, often depicting products or places with captions that, while semantically clear, may contain noise such as SEO keywords. The dataset was assembled using an existing CLIP model to filter CommonCrawl data, focusing on images with alt-text for creating pairs. Preprocessing involved removing pairs with low cosine similarity between text and image embeddings, leading to a significant reduction from the initial collection. LAION-5B facilitates training state-of-the-art language-vision models, offering unprecedented scale for research into zero-shot transfer, robustness, and multimodal learning.

    \item \href{https://laion.ai/blog/laion-coco/}{\textbf{LAION-COCO}}~\cite{schuhmann2022laion}.
    LAION-COCO is a dataset featuring 600 million synthetic captions for images from the LAION-5B English subset, utilizing models like BLIP L/14 and CLIP. It was developed to explore the potential of generated captions in training models. The dataset includes the original and top captions alongside alternative ones, all available in parquet files. This unique assembly allows for the examination of synthetic captions' impact on model training, offering a vast resource for multimodal learning. 
    
    \item \href{https://github.com/kakaobrain/coyo-dataset}{\textbf{COYO-700M}}~\cite{kakaobrain2022coyo-700m}. 
    The COYO-700M dataset comprises 747 million image-text pairs, meticulously curated from CommonCrawl data spanning from October 2020 to August 2021, designed to enhance multimodal learning in vision-and-language research. This extensive collection targets the informative association between alt-text and corresponding images in HTML documents, undergoing rigorous image and text-level filtering to boost quality, reduce redundancy, and eliminate inappropriate content. Tailored for training large-scale foundation models, COYO-700M supports diverse image formats and offers a variety of meta-attributes, making it a crucial resource for advancing machine learning models and applications, particularly in tasks like image captioning and visual question answering. This dataset represents a significant stride in understanding the complex relationship between visual and textual data, facilitating the development of more sophisticated vision-and-language models.
    
    \item \href{https://www.datacomp.ai/}{\textbf{DataComp}}~\cite{gadre2024datacomp}. 
    The DataComp challenge provides a testbed for image-text datasets. The dataset proposed in this challenge, known as COMMONPOOL, is a large-scale multimodal dataset constructed from 12.8 billion image-text pairs sourced from Common Crawl, designed to foster innovation in dataset design within the machine learning community. This challenge allows researchers to participate in two tracks: filtering from the provided pool COMMONPOOL datasets or using external data in a "Bring Your Own Data" (BYOD) approach, ensuring data does not overlap with evaluation sets. This approach aims to enhance the understanding of how dataset curation impacts machine learning model performance, placing a strong emphasis on rigorous dataset design over algorithmic competition.

    \item \href{https://www.cs.rice.edu/~vo9/sbucaptions/}{\textbf{SBU}}~\cite{ordonez2011im2text}.
    The SBU captioned photo dataset features over 1 million Flickr images, each with a user-generated caption, developed to bridge visual content with natural language descriptions. This extensive collection is the result of targeted Flickr queries and careful filtering to ensure captions accurately reflect the visual elements of the images. The dataset facilitates the challenging task of automatic image description using simple matching techniques and the incorporation of various image content estimates like objects, attributes, and scenes. This approach has shown promising results in non-parametric image captioning methodologies. Moreover, the SBU dataset introduces a novel performance measure for evaluating image captions, providing a valuable resource for research in automated image understanding and description generation. With its focus on leveraging web-sourced captions for detailed image annotation, the SBU dataset represents a significant advancement in the field of image captioning.
    
    \item \href{https://ai.google.com/research/ConceptualCaptions/}{\textbf{Conceptual Captions 3M (CC3M)}}~\cite{sharma2018conceptual}.
    The Conceptual Captions (CC3M) dataset is constructed by programmatically harvesting and processing image-caption pairs from billions of web pages, focusing on alt-text associated with images. This process includes rigorous filtering based on image quality, relevance, and caption appropriateness, followed by text transformations where specific names and details are generalized to create more universally learnable captions. Comprising approximately 3.3 million pairs, the CC3M dataset is designed to be significantly larger and more diverse than traditional datasets like MS-COCO. 
    % Its purpose is to enhance the development and effectiveness of image captioning models by providing a vast and varied set of training data, which can be used in applications such as aiding visually impaired individuals and improving image retrieval systems.
    
    \item \href{https://ai.google.com/research/ConceptualCaptions/}{\textbf{Conceptual Captions 12M (CC12M)}}~\cite{changpinyo2021conceptual}. The CC12M dataset was created by relaxing filters used in the CC3M dataset, resulting in a larger set of 12 million image-text pairs for vision-and-language pre-training. This dataset exhibits a longer-tail distribution, capturing a wider range of visual concepts compared to CC3M. By including more diverse and complex concepts, CC12M aims to improve transferability and performance on long-tail recognition tasks in vision-and-language models. The dataset's creation process involved steps such as image-based and text-based filtering, as well as text transformations to enhance privacy and maintain data quality. Overall, CC12M serves as a valuable resource for addressing challenges in vision-and-language tasks, offering a rich and diverse set of training examples for improved model generalization and performance.

    \item \href{https://wukong-dataset.github.io/wukong-dataset/}{\textbf{Wukong}}~\cite{gu2022wukong}.
    The Wukong dataset, containing 100 million Chinese image-text pairs from the web, is significant for Chinese vision-language pre-training (VLP) models. Its preprocessing includes image and text-based filters to ensure quality: images are screened for size and aspect ratio, while texts are checked for language, length, and relevance, discarding overly common or irrelevant descriptions. This careful curation addresses the lack of large-scale Chinese datasets, facilitating the development and benchmarking of VLP models across diverse concepts and applications. 

    \item \href{}{\textbf{ALT200M}}~\cite{hu2022scaling}.
    The ALT200M dataset comprises over 200 million image-text pairs sourced from the web, using image alt attributes. Constructed to explore scaling in vision-language pre-training (VLP) for image captioning, the dataset aims to assess the impact of increased model and data sizes on VLP performance. Images and corresponding alt-texts were collected via a pipeline with minimal rule-based filtering, focusing on image size and aspect ratio, while alt-texts were curated based on length and vocabulary derived from English Wikipedia. Named entities in texts were anonymized to maintain privacy. The dataset is designed to facilitate experiments on various model sizes and configurations, particularly in handling large-scale, noisy data, with the goal of improving recognition of diverse and rare visual concepts and achieving new benchmarks in image captioning.

    \item \href{}{\textbf{LTIP}}~\cite{alayrac2022flamingo}.
    The Long Text \& Image Pairs (LTIP) dataset, consisting of approximately 312 million image and text pairs, is meticulously assembled from various web sources to ensure high-quality and lengthy textual descriptions, surpassing typical datasets in detail. This dataset serves as a fundamental component in training the Flamingo models, which are tailored for multimodal tasks involving both visual and textual data interpretation. Through rigorous quality checks and careful formatting, LTIP is optimized for integration into training systems, significantly enhancing the capability of models like Flamingo to perform complex vision and language tasks. The primary purpose of the LTIP dataset is to enrich these models' understanding and generation of contextually relevant textual descriptions from visual inputs, thereby boosting their efficacy across diverse vision and language applications.
    
\end{itemize}
\paragraph{Content Descriptive Image-Caption Datasets.} Content descriptive image-caption datasets contain longer caption with more descriptive information. Usually each image in content description image-caption datasets contain at least 5 sentences of caption.
\begin{itemize}
    \item \href{https://cocodataset.org/}{\textbf{MS-COCO}}~\cite{chen2015microsoft}. This dataset contains 328k images with a total of 2.5 million labeled instances, the creation of this dataset drew upon extensive crowd worker involvement via novel user interfaces for category detection, instance spotting and instance segmentation. The MS-COCO dataset was created by collecting images from Flickr that contain multiple objects in their natural context, with captions gathered through human subjects on Amazon's Mechanical Turk. Each image has multiple reference captions, with a subset having 40 reference sentences to improve evaluation metrics' correlation with human judgment. The dataset includes training, validation, and testing sets. This dataset's characteristics make it suitable for training and evaluating algorithms for image captioning tasks, addressing the challenge of generating accurate and descriptive captions for diverse and complex visual content of existing LLMs.

    \item \href{https://shannon.cs.illinois.edu/DenotationGraph/}{\textbf{Flickr30K}}~\cite{young2014image}. The Flickr30K dataset in the article was created by collecting 31,783 images depicting everyday activities and events from Flickr, along with 158,915 captions obtained through crowd-sourcing. This dataset extends a previous corpus and follows similar annotation guidelines to ensure quality control. Each image is described by five annotators, providing diverse descriptions ranging from general situations to specific actions. The dataset's unique feature lies in the variety of descriptions associated with each image, enabling the induction of denotational similarities between expressions not directly related by syntactic rules. This dataset can be utilized to address challenges in semantic inference tasks by leveraging the visual denotations of linguistic expressions to define novel similarity metrics and enhance understanding of textual descriptions in relation to visual content.

    \item \href{}{\textbf{WEBLI}}~\cite{chen2022pali}.
    The WEBLI dataset is a vast multilingual image-language dataset comprising 10 billion images and approximately 12 billion alt-texts, constructed from publicly available internet resources to support the training of the PaLI multimodal model. It includes text in over 100 languages and features OCR annotations to enhance text recognition capabilities in images. To ensure high quality, only the top 10\% of image-text pairs, totaling around 1 billion, were retained for training the PaLI model. The dataset's primary purpose is to facilitate the pre-training of large-scale models on a variety of multimodal tasks across multiple languages, thereby improving the models' performance on complex tasks such as image captioning and visual question answering, and advancing research in image and language processing.

    \item \href{}{\textbf{ALIGN}}~\cite{jia2021scaling}.
    The ALIGN dataset represents a significant expansion over CC3M by utilizing over one billion image-text pairs, compared to CC3M's 3.3 million. This increase is achieved by simplifying the data collection process; while CC3M underwent rigorous image-based, text-based, and image\&text-based filtering to ensure high-quality data, ALIGN limits its preprocessing to only image-based and text-based filtering. By omitting the image\&text-based filtering step, ALIGN trades some data cleanliness for scale, demonstrating that the volume of data can outweigh the impact of noise. This approach facilitates the training of more robust models capable of understanding complex visual and linguistic tasks, highlighting a strategic shift towards leveraging the vast, albeit imperfect, data available on the web for advanced representation learning.

    \item \href{https://github.com/lichengunc/refer}{\textbf{RefCOCOg}}~\cite{yu2016modeling, mao2016generation}.
    RefCOCOg is a dataset created through Amazon Mechanical Turk, featuring 85,474 natural language referring expressions for 54,822 objects across 26,711 MSCOCO images. Images were chosen to have 2 to 4 objects of the same category, ensuring complexity in object referencing. The dataset's creation involved two sets of workers: one to write expressions for objects in images and another to identify objects based on these expressions. Validity was confirmed through successful object identification, making RefCOCOg a robust resource for tasks requiring detailed understanding of complex, referential language in visual contexts.
	
    \item \href{https://github.com/lichengunc/refer}{\textbf{RefCOCO \& RefCOCO+}}~\cite{kazemzadeh2014referitgame, mao2016generation,yu2016modeling}.
    RefCOCO and RefCOCO+ are datasets generated through the ReferItGame, a two-player game designed to collect natural language expressions referring to objects within images. RefCOCO contains 142,209 expressions for 50,000 objects in 19,994 images. RefCOCO+ includes 141,564 expressions for 49,856 objects across 19,992 images, specifically banning location words in expressions to focus on appearance-based descriptions. This approach aims to gather expressions independent of viewer perspective, providing a rich resource for computer vision tasks requiring detailed object identification based on descriptive language.
    
    \item \href{https://homes.cs.washington.edu/~ranjay/visualgenome/index.html}{\textbf{Visual Genome}}~\cite{krishna2017visual}.
    The Visual Genome dataset vastly enhances the scope of image-text pair research, offering over 108,000 images enriched with detailed annotations, a leap from CC3M's 3.3 million pairs. It diverges from CC3M's simpler image-caption pairs by integrating images from the YFCC100M and MS-COCO datasets, supplemented with extensive crowd-sourced annotations. Beyond mere captions, it details over 3.8 million object instances, attributes, and object relationships within images through structured scene graphs. This innovation not only expands the dataset's volume but also its utility for advanced image understanding, providing a comprehensive framework for analyzing complex visual scenes. Visual Genome aims to advance the field by enabling models to interpret nuanced visual contexts, making it a pivotal resource for progressing in object detection, scene comprehension, and visual reasoning. In essence, Visual Genome represents a significant evolution in image-text datasets, designed to mirror the complexity of the visual world.

    \item \href{https://huggingface.co/datasets/liuhaotian/LLaVA-Pretrain}{\textbf{CC595k}}~\cite{liu2024visual}.
    The CC595k dataset is derived from the CC3M dataset, refined to include around 595,000 image-text pairs. This selection process involved extracting noun-phrases from captions, focusing on those with a frequency of at least 3 to ensure concept coverage while omitting rare phrases. For highly frequent noun-phrases (over 100 occurrences), a random subset of 100 captions was chosen. This preprocessing aims to balance concept variety against the dataset's size, optimizing for broad yet manageable representation of concepts within the constraints of fewer image-text pairs.

    \item \href{https://textvqa.org/textcaps/}{\textbf{TextCaptions}}~\cite{sidorov2020textcaps}. The TextCaps dataset was created with the aim of exploring the task of image captioning with reading comprehension. The dataset collection involved annotators describing images in one sentence that required reading the text present in the image. The dataset contains 145,329 captions for 28,408 images, with a focus on integrating OCR tokens into image descriptions. Annotators were tasked with generating captions that relate text to visual context, requiring spatial, semantic, and visual reasoning. This dataset presents new technical challenges for existing image captioning models, as it requires understanding and incorporating text from images into descriptive sentences. The TextCaps dataset can be used to address the challenge of teaching image captioning models how to "read" and process information from text within images, potentially benefiting visually impaired individuals and advancing AI research in image understanding tasks.

    \item \href{https://github.com/nocaps-org}{\textbf{NoCaps}}~\cite{agrawal2019nocaps}.
    The Nocaps dataset enhances image captioning with 166,100 captions for 15,100 images from the Open Images Dataset V4, focusing on objects not in COCO Captions, including nearly 400 novel objects. Images, primarily from Flickr, are categorized into in-domain, near-domain, and out-of-domain, based on their object classes' relation to COCO, to test model generalization across familiar and novel concepts. Developed with AMT captions, the dataset introduces a "priming" method for more accurate descriptions by hinting at object categories during annotation. This large-scale, diverse dataset aims to bridge the gap between existing captioning datasets and the vast array of real-world visual concepts, providing a challenging benchmark for novel object captioning. Nocaps dataset pushes image captioning models towards broader visual comprehension and linguistic description capabilities, aiming for applicability in more generalized, real-world scenarios.

    \item \href{https://vizwiz.org/tasks-and-datasets/image-captioning/}{\textbf{VizWizCap}}~\cite{gurari2020captioning}.
    The VizWizCap dataset, also known as VizWiz-Captions, comprises over 39,000 images taken by people who are blind, each annotated with five captions to facilitate research in image captioning algorithms that better serve blind users. Constructed using crowdsourced captions from the Amazon Mechanical Turk platform, this dataset includes metadata on text presence and image quality, reflecting real-world variability in the images. The primary purpose of the VizWizCap dataset is to advance the development of image captioning technology by providing a resource that addresses the specific needs of blind individuals, challenging existing computer vision models with images that significantly differ from those in controlled environments typically found in other datasets. This initiative aims to bridge technological gaps and enhance the practical utility of assistive technologies for visually impaired users.

    \item \href{https://github.com/AIChallenger/AI_Challenger_2017}{\textbf{AI Challenger Captions}}~\cite{wu2017ai}. 
    The AI Challenger dataset was created to address the limitations of existing image caption datasets labeled in English. It is the largest image captioning dataset with Chinese annotations, consisting of three sub-datasets: human keypoint detection, large-scale attribute dataset, and image Chinese captioning. The dataset aims to bridge the semantic gap between low-level images and high-level concepts by providing rich annotations such as class labels, keypoint coordinates, bounding boxes, attributes, and captions in Chinese. This dataset not only serves as an effective benchmark for evaluating and improving computational methods in image understanding but also offers a valuable resource for researchers and practitioners working on tasks related to image understanding.

    \item \href{https://visionandlanguage.net/VIST/}{\textbf{VIST}}~\cite{huang2016visual}.
    The VIST dataset pioneers sequential vision-to-language learning by offering 81,743 unique photos across 20,211 sequences, aimed at visual storytelling. Derived from Flickr, it's structured into three tiers: isolated image descriptions (DII), sequential image descriptions (DIS), and image sequence stories (SIS), enriched by crowdsourced annotations from Amazon Mechanical Turk. This tiered approach enables the study of narrative and temporal context effects on visual comprehension. The dataset underwent careful preprocessing, including tokenization and anonymization, to ensure consistency and privacy. An automatic evaluation metric, grounded in METEOR scores, benchmarks storytelling performance, aligning closely with human judgment. "VIST" significantly advances AI's capability to not just describe but narrate visual sequences, enhancing machines' understanding and generation of human-like stories from visual data, marking a leap towards more nuanced and context-aware AI storytelling abilities.
    
\end{itemize}

\paragraph{Interleaved Image-Text Document Datasets}
Interleaved image-text document datasets consist of a text document interspersed with several illustrative images, wherein the correlation between the images and the accompanying text tends to be relatively lower.
\begin{itemize}
    \item \href{https://figshare.com/articles/dataset/MW3-Dataset/22154066/3}{\textbf{M3W}}~\cite{alayrac2022flamingo}.
    The M3W dataset (MultiModal MassiveWeb dataset), derived from about 43 million webpages, is crafted for training Flamingo on interleaved text and image data. It features data from the Document Object Model (DOM) of webpages, with <image> tags inserted in plain text at their original positions, followed by a special <EOC> token for delineation. To ensure manageability and diversity, from each document, a sequence of 256 tokens and up to the first 5 images are selected, discarding the rest. The dataset emphasizes clean, non-English, and explicit content-free data, using custom scrapers for content extraction that maintains the hierarchical structure of HTML. It undergoes rigorous preprocessing, including text filtering to eliminate low-quality documents and image filters to remove unsuitable visuals. M3W is instrumental for developing few-shot learning in models, enabling them to perform complex image and video tasks with minimal examples, thereby serving as a key resource for advancing multimodal machine learning. This dataset is not open-source, luckily, the Open Flamingo provide an alternative open-source dataset called MMC4.

    \item \href{https://github.com/allenai/mmc4}{\textbf{MMC4}}~\cite{zhu2024multimodal}. 
    The Multimodal C4 (MMC4) dataset is constructed as a significant enhancement of the well-known text-only C4 corpus, incorporating images alongside text to foster advancements in in-context vision and language models. The construction of the dataset involves several meticulous steps, leveraging the public web pages contained in the cleaned English C4 corpus as the primary source. The process includes standard preprocessing methods like deduplication, NSFW (not safe for work) image removal, ad filtering, and more. Images are placed into text sequences using a linear assignment algorithm based on CLIP features, a method that showed superiority over alternatives in aligning images to relevant textual content. After these filtration processes, the final MMC4 dataset comprises over 101.2 million documents, featuring 571 million images interleaved within 43 billion English tokens. The Multimodal C4 (mmc4) dataset is designed to advance the capabilities of in-context vision and language models, enabling them to understand and process interleaved sequences of images and text. 

    \item \href{https://huggingface.co/datasets/HuggingFaceM4/OBELICS}{\textbf{OBELICS}}~\cite{laurenccon2024obelics}.
    The OBELICS dataset is a meticulously constructed, open web-scale filtered dataset comprising 141 million web pages, 353 million images, and 115 billion text tokens derived from the Common Crawl dumps. Designed to advance the training of large multimodal models, it addresses the scarcity of publicly available datasets by providing a rich collection of interleaved image-text documents. The construction process encompasses several key steps: collecting and simplifying HTML files, extracting and filtering multimodal web documents, and implementing responsible filtering and deduplication measures to ensure quality and minimize inappropriate content. By preserving the natural structure of web documents and emphasizing the contextual interplay between text and images, OBELICS aims to support the development of next-generation models capable of sophisticated understanding and generation of multimodal content, thereby filling a critical gap in resources available for multimodal research and model training.
\end{itemize}

\paragraph{Visual Question Answer Image-Caption Datasets.} These datasets are usually driven by asking question on the image and giving out the answer according to the character of the image. Usually each image in this kind of datasets contains one question and one short answer as its caption.
\begin{itemize} 
    \item \href{https://visualqa.org/}{\textbf{VQAv2.0}}~\cite{goyal2019making}. 
    VQAv2.0 is a new dataset aiming to help with the problem in understanding pictures and answering questions about them, known as Visual question answering(VQA)~\cite{antol2015vqa} problem. The VQA2.0 dataset contains approximately 1.1 million image-question pairs, almost twice the size of the original VQA dataset. It includes around 13 million answers associated with roughly 200,000 images from the COCO dataset. The dataset is divided into train, validation, and test splits, with complementary images and answers collected for all splits. The VQA2.0 dataset was constructed by adding "complementary" images to the existing VQA dataset. For each question-answer pair associated with an original image, a similar yet distinct image was selected, where the same question would have a different answer. This approach resulted in a dataset where each question is linked with two images, leading to two different answers, thereby doubling the number of image-question pairs. This method aimed to balance the dataset and reduce the inherent biases towards certain answers. The complementary images were identified through a data collection protocol involving human annotators who selected images from a set of nearest neighbors (based on deep features) that were visually similar to the original image but would lead to a different answer to the same question.
    
    \item \href{https://ai.stanford.edu/~yukez/visual7w/}{\textbf{Visual-7W}}~\cite{zhu2016visual7w}.
    Visual-7W enriches COCO images with 327,939 QA pairs, linked via object-level annotations to 47,300 images, covering what, where, when, who, why, how, and which questions. Questions and answers were generated through Amazon Mechanical Turk, where workers were asked to create natural language expressions for objects and another set to identify objects based on these expressions. This dual-step process ensures high-quality, relevant textual descriptions, directly tied to image regions. Visual-7W is a leap towards models that understand both the visual and textual components of an image, offering a robust platform for advanced AI research.

    \item \href{https://rrc.cvc.uab.es/?ch=11}{\textbf{ST-VQA}}~\cite{biten2019scene}. 
    The ST-VQA dataset creation process involved collecting images from various datasets containing scene text and other computer vision data sources. The ST-VQA dataset, incorporating 23,038 images from diverse sources like ICDAR, ImageNet, VizWiz, Visual Genome, and COCO-Text, focuses on integrating textual information within images for answering questions. Questions and answers were crowd-sourced through Amazon Mechanical Turk, ensuring unambiguous answers based on text in the images. The dataset comprises 23,038 images with 31,791 question-answer pairs for training and testing. ST-VQA emphasizes leveraging high-level semantic information from text in images for visual question answering tasks. It addresses the challenge of reasoning and generating answers based on scene text, providing a unique dataset for exploring the integration of textual cues in the VQA process.

    \item \href{https://github.com/shikras/shikra}{\textbf{Shikra-RD}}~\cite{chen2023shikra}.
    Shikra-RD is a dataset generated using GPT-4 to annotate Flickr30K Entities images with relational descriptions (RD), focusing on objects identified within bounding boxes. Despite GPT-4's inability to view images, it interprets them through detailed descriptions and bounding box formats to create Q\&A pairs, emphasizing questions that leverage known information for answers. This process resulted in 5,922 QA pairs, including coordinate data. Shikra-RD, leveraging advanced language models for image understanding, aims to enrich RD datasets by incorporating spatial annotations and natural language questions and answers.

    \item \href{https://ocr-vqa.github.io/}{\textbf{OCR-VQA}}~\cite{mishra2019ocr}.
    OCR-VQA consists of 207,572 book cover images, 1 million QA pairs, designed for reading text in images through OCR. The dataset emphasizes visual question answering (VQA) by incorporating optical character recognition (OCR) to interpret text on book covers for answering questions. QA pairs are derived from metadata and human paraphrasing of template questions, addressing titles, authors, genres, etc. The dataset, with its unique focus on text reading within VQA, poses challenges in text detection and recognition, aiming to advance both document analysis and VQA research fields.

    \item \href{https://www.docvqa.org/}{\textbf{DocVQA}}~\cite{mathew2021docvqa}.
    The DOC-VQA dataset, encompassing over 50,000 questions on more than 12,000 document images, was annotated through a meticulous three-stage process using a web-based tool and the efforts of remote workers. Workers initially generated question-answer pairs directly from text present in the images, aiming for extractive QA akin to NLP and VQA tasks. Subsequent stages involved verification and refinement of these QAs, including assigning question types and ensuring the precision of answers. This process underscores DOC-VQA's commitment to high-quality, relevant, and diverse annotations for advancing document-based VQA research.

    \item \href{https://allenai.org/project/a-okvqa/home}{\textbf{A-OKVQA}}~\cite{marino2019ok}. The A-OKVQA dataset was created by generating a diverse set of about 25K questions that require a broad base of commonsense and world knowledge to answer. Unlike existing knowledge-based VQA datasets, the questions in A-OKVQA cannot be answered simply by querying a knowledge base; instead, they demand some form of commonsense reasoning about the scene depicted in the image. This dataset aims to push the boundaries of Visual Question Answering by requiring models to recognize the image, understand the question, recall relevant knowledge, and use reasoning to arrive at an answer. It serves as a challenging testbed for AI models to reason over visual and natural language inputs, addressing the need for more complex reasoning systems in VQA tasks.

    \item \href{https://textvqa.org/}{\textbf{TextVQA}}~\cite{singh2019towards}.
    The Text-VQA dataset comprises 28,408 images with 45,336 questions requiring textual information within images to answer. Sourced from Open Images, the dataset spans categories likely to include text, aiming to enhance VQA models' text-reading capabilities. Questions and answers were collaboratively generated using a web-based annotation tool by remote workers in a three-stage process, ensuring the questions necessitate text interpretation for answers. This dataset pushes the boundaries of VQA by demanding models to not only perceive images but also read and comprehend text within them, marking a significant step towards models assisting in real-world tasks, particularly aiding visually impaired users. 

    \item \href{https://cs.stanford.edu/people/dorarad/gqa/about.html}{\textbf{GQA}}~\cite{hudson2019gqa}.
    The GQA dataset is designed to address deficiencies in previous visual question answering (VQA) datasets by fostering advanced visual reasoning and reducing biases. It utilizes over 22 million questions generated from 113K real-world images annotated with detailed scene graphs, detailing objects, attributes, and relationships. Each question is crafted through a robust engine combining linguistic grammar with scene graph data, and is accompanied by a functional program that semantically represents the reasoning steps needed for answering, ensuring complexity and diversity. GQA also introduces new metrics for evaluating consistency, validity, plausibility, and grounding of responses, moving beyond simple accuracy to offer a more comprehensive assessment of AI models' visual and compositional understanding. This dataset aims to promote the development of AI capabilities in deep semantic understanding and unbiased reasoning in visual contexts.

\end{itemize}

% \paragraph{Image-text dialog datasets}
% \begin{itemize}
%     \item \href{https://github.com/victorsungo/MMDialog}{\textbf{MMDialog}~\cite{feng2022mmdialog}.}
%     The MMDialog dataset is a comprehensive multi-modal dialogue dataset compiled from real social media interactions, containing 1.08 million dialogue sessions and 1.53 million images across 4,184 topics. It is designed to enhance the development of conversational agents that can process and respond with both textual and visual information. With an average of 2.59 images and 4.56 turns per dialogue session, this dataset is structured to mimic real-world interactions, supporting research on multi-modal communication. It provides baseline models and novel evaluation metrics, fostering advancements in conversational AI by facilitating the study of more natural and engaging user interactions in open-domain settings.

%     \item \href{https://arxiv.org/abs/1910.05728}{\textbf{VisDial}}~\cite{patro2019granular}
% \end{itemize}

\paragraph{Domain-Specific Image-Caption Datasets.}
Domain-specific image-caption datasets are collections of images paired with captions that are tailored to a particular field or industry. It can enhance the performance of LLMs in specific domains.
\begin{itemize}
    \item \href{https://github.com/google-research-datasets/screen2words}{\textbf{Screen2Words}}~\cite{wang2021screen2words}.
    The Screen2Words dataset is designed to advance the automatic summarization of mobile user interfaces (UIs), encompassing 22,417 unique Android UI screens derived from the RICO dataset. This dataset is annotated by professional labelers, yielding 112,085 language summaries aimed at capturing the core functionalities of each screen for applications in screen readers, conversational agents, and other language-based interfaces. It supports multi-modal learning, leveraging text, images, and UI structure to enhance semantic understanding and interaction. The primary goal is to foster research in HCI and machine learning to improve accessibility and usability, making it easier for systems to provide concise, useful descriptions of mobile UIs automatically.

    \item \href{https://github.com/google-research-datasets/widget-caption5}{\textbf{WidgetCap}}~\cite{li2020widget}.
    The WidgetCap dataset aims at enhancing mobile UI accessibility by generating descriptions for UI elements. It comprises 162,859 human-annotated captions for 61,285 UI elements across 21,750 screens from 6,470 apps, sourced from the RICO dataset and manually annotated via Amazon Mechanical Turk. This initiative addresses the prevalent issue of missing UI captions, crucial for accessibility and voice interactions. The dataset's multimodal nature, combining image and structural UI data, enables comprehensive model training for accurate caption generation. WidgetCap's creation process involved rigorous preprocessing to ensure data quality, focusing on visible and clickable elements essential for interaction. By providing a vast resource for widget captioning, WidgetCap facilitates research and development towards more accessible and interactive mobile applications, representing a significant stride in bridging accessibility gaps in mobile UI design.

\end{itemize}

%%%%%%%%%%%%%%%%%5
\subsubsection{Video-Caption Datasets}\label{sec:appen:datasets:video_datasets}
In this subsubsection, we provide a comprehensive summary of video caption datasets to help people find the most suitable datasets for MLLMs training.
\begin{itemize}
    \item \href{https://www.microsoft.com/en-us/research/publication/msr-vtt-a-large-video-description-dataset-for-bridging-video-and-language/}{\textbf{MSR-VTT}}~\cite{xu2016msr}.
    Microsoft Research Video-to-Text (MSR-VTT) is a large-scale dataset offering 10,000 video clips totaling 41.2 hours, accompanied by 200K clip-sentence pairs. 
    Derived from 257 queries across 20 categories, the dataset ensures diversity and representativeness for training large parameter models. 
    MSR-VTT is meticulously curated, involving the collection of 30,404 videos from top search results, clip selection based on shot segmentation, and sentence annotation by Amazon Mechanical Turk workers. 
    Noteworthy adopters of MSR-VTT include Git~\cite{wang2022git}, Vatt~\cite{akbari2021vatt}, Videoclip~\cite{xu2021videoclip}, Lavis~\cite{li2022lavis}, and TVLT~\cite{tang2022tvlt}, showcasing its significance in language-video research.
    
    \item \textbf{WebVid 2M, WebVid 10M}~\cite{bain2021frozen}.
    The WebVid dataset originally encompasses 2.5 million video clips collected from various web sources, each paired with a caption, and subsequently expands to encompass 10 million pairs of video and text totaling 13k hours.
    Scraped from web sources similar to the image-text dataset Google Conceptual Captions~\cite{sharma2018conceptual} (CC3M), WebVid offers diverse video content with text descriptions, adhering to ethical processing standards for copyright compliance.
    The textual descriptions in WebVid are typically manually crafted, allowing for better alignment with the content of the video images due to the well-structured sentences, fewer grammatical errors, and richer vocabulary. 
    Adopted by models like Stable Video Diffusion~\cite{blattmann2023stable}, Next-gpt~\cite{wu2023next} and Videochat~\cite{li2023videochat}, WebVid serves as a valuable resource for text-to-video generation task. However, because of the copyright, WebVid is no longer available.
    
    \item \href{https://github.com/lucidrains/flamingo-pytorch}{\textbf{VTP}}~\cite{alayrac2022flamingo}.
    VTP (Video \& Text Pairs) consists of 27 million short videos paired with descriptive sentences, collected by crawling less than ten websites known for high-quality and detailed video descriptions. 
    Each instance within the dataset consists of a sequence of UTF-8 bytes encoding the textual content and a compressed video.
    VTP is processed in a manner including adding image labels and special tokens.
    Additionally, automated text formatting is applied to eliminate irrelevant information, such as dates and locations, from the captions, thus refining the dataset for training purposes.
    Notably, deduplication is omitted due to the unique sourcing strategy of this dataset, ensuring minimal overlap with common video evaluation datasets.
    VTP is leveraged by models such as Flamingo~\cite{alayrac2022flamingo} for few-shot Learning.

    \item \href{https://snap-research.github.io/Panda-70M/}{\textbf{Panda70M}}~\cite{chen2024panda}.
    The Panda-70M dataset was created through an automatic captioning pipeline that leverages multimodal information, such as video descriptions, subtitles, and individual static video frames. This dataset contains high-resolution and semantically coherent video samples, aiming to provide precise descriptions of the main objects and actions in the videos. The dataset addresses the limitations of existing datasets by offering a large-scale collection of videos with annotations generated by multiple cross-modality vision-language models. It can be utilized to enhance various downstream tasks, including video captioning, video and text retrieval, and text-to-video generation.
\end{itemize}

\subsubsection{Audio-Caption Datasets}\label{sec:appen:datasets:audio_datasets}
In this subsubsection, we provide a comprehensive summary of audio caption datasets to help people find the most suitable datasets for MLLMs training.
\begin{itemize}
    \item \href{https://github.com/kaldi-asr/kaldi/tree/master/egs/aishell2}{\textbf{AISHELL-2}}~\cite{du2018aishell}.
    AISHELL-2 is a Mandarin Chinese Speech Corpus containing 1000 hours of clean speech data from 1991 Chinese speakers across diverse regions. This dataset covers 12 domains including keywords, voice commands, smart home, autonomous driving and industrial production, etc. The data was recorded in a quiet indoor environment using the iOS-system. Through professional speech annotation and strict quality inspection, the manual transcription accuracy rate of this dataset is above 96\%.
    
    \item \href{https://github.com/XinhaoMei/WavCaps}{\textbf{WavCaps}}~\cite{mei2023wavcaps}.
    WavCaps is a large-scale English audio captioning dataset that offers a vast collection of around 400k audio clips, each paired with corresponding captions. The dataset is sourced from three prominent websites, including FreeSound~\cite{font2013freesound}, BBC Sound Effects~\footnote{https://sound-effects.bbcrewind.co.uk/}, and SoundBible~\footnote{https://soundbible.com/}, along with a sound event detection dataset AudioSet Strongly-labelled Subset~\cite{hershey2021benefit}. To ensure high data quality, the dataset undergoes a three-stage processing pipeline, which can filter and convert the raw descriptions obtained from the aforementioned sources into accurate and informative captions using ChatGPT~\footnote{https://pypi.org/project/langdetect/}.
    
    \item \href{https://x-llm.github.io/}{\textbf{VSDial-CN}}~\cite{chen2023x}.
    VSDial-CN is a multi-modal Automatic Speech Recognition (ASR) dataset constructed from VisDial~\cite{das2017visual}. It comprises around 120,000 images, each accompanied by a caption and 10 rounds of dialogue consisting of questions and answers. To create VSDial-CN, the text from the VisDial dataset was translated into Chinese, and the questions were then synthesized into speech using the FastSpeech2~\cite{ren2020fastspeech} model. The dataset offers approximately 1,200k training samples for multimodal ASR. After removing duplicate questions, there are approximately 370k unique speech utterances available for training.
    
\end{itemize}

\subsubsection{3D-Caption Datasets.}\label{sec:appen:datasets:3d_datasets}
\begin{itemize}
    \item \href{https://github.com/ScanNet/ScanNet}{\textbf{ScanNet}}~\cite{dai2017scannet}. With a substantial scale comprising 2.5 million views across 1513 scenes, ScanNet offers RGB-D video data annotated with 3D camera poses, surface reconstructions, and semantic segmentations. ScanNet, which is a snapshot of available data from roughly one month of data acquisition by 20 users at locations in several  countries, incorporates annotations from over 500 crowd workers via the Mechanical Turk platform. Its creation involved a meticulous process encompassing data collection, RGB-D scanning and calibration, data upload and processing, semantic annotation, and dataset organization.
    Notably, a data collection framework was designed to enable untrained users to capture semantically labeled indoor scenes using commercial hardware. The captured RGB-D videos underwent rigorous processing stages, including calibration to align depth data with color data, surface reconstruction, camera attitude estimation, and quality verification. Semantic annotation, performed through crowdsourcing, involved instance-level object class labeling and CAD model alignment tasks.
    ScanNet has been included in the pytorch library Kaolin and adopted by models such as ENet, FCAF3D, PointNet++.
    % ScanNet is pivotal for advancing research in understanding 3D environments.

    \item \href{http://buildingparser.stanford.edu/dataset.html}{\textbf{S3DIS}}~\cite{armeni2017joint}. S3DIS provides a comprehensive collection of indoor scene point clouds. S3DIS encompasses six large-scale indoor areas with a total of 271 rooms, with each point in the scene point cloud annotated with one of the 13 semantic categories.
    Point clouds are automatically generated using the Matterport scanner without any human intervention, sets of RGB-D images registered on color point clouds was collected to enrich the dataset.
    Point cloud data was further processed to parse the building's 3D point clouds into semantically meaningful spaces like rooms, which were then subdivided into structural and architectural elements like walls and columns. 
    This involved using a 3D sliding window-based approach and machine learning techniques for semantic element detection and labeling. The application of graph models enhanced the context consistency between elements, facilitating effective extraction and understanding of semantic information in complex indoor spatial point clouds.
    S3DIS has been adopted by models including FCAF3D, PointNet, and PointCNN.

    \item \href{https://structured3d-dataset.org/}{\textbf{Structured3D}}~\cite{zheng2020structured3d}. Structured3D is a comprehensive collection of 3,500 home designs with 21,835 rooms, derived from a large database of house designs meticulously created by professional designers. It includes detailed information on interior design elements in industry-standard format, detailing object geometry, materials, textures, and functional information like room assignments. An automated program was developed to extract geometric primitives related to room structure, including ceilings, floors, walls, and openings, from a large database of house designs hand-crafted by professional designers. Precise measurements and related information are used to construct detailed models, including all planes, lines, connections, and their relationships.
    For the creation of photorealistic 2D renderings, the dataset utilizes a specialized rendering engine that employs ray tracing method to approximate the real global lighting effect for RGB rendering. The rendering process uses over a million CAD furniture models from leading manufacturers. Furthermore, default lighting Settings are provided and images with different visual effects are generated by adjusting furniture configurations and lighting Settings. The dataset has been adopted by models such as Structured3D, Ponder V2, and Swin3D.
\end{itemize}

%%%%%%%%%%%%%%%%%%%%%%%%%%%%%%%%%%%%%%%

\subsection{Commonly-Used Instruction Tuning Datasets}\label{sec:appen:it}
Instruction tuning datasets are used to fine-tune models to better understand and follow specific instructions, improving their ability to generate accurate and relevant responses. These datasets help enhance the model's performance in various tasks by providing it with clear and structured examples of desired outputs based on given inputs. We summarize the commonly used multimodal instruction tuning datasets here.
\subsubsection{Image instruction tuning datasets}\label{sec:appen:it:image}
In this subsubsection, we provide a comprehensive summary of image instruction tuning datasets to help people find the most suitable datasets for visual instruction tuning.
\begin{itemize}
    \item \href{https://huggingface.co/datasets/liuhaotian/LLaVA-Instruct-150K}{\textbf{LLAVA-Instruct-150K}}~\cite{liu2024visual,liu2023improved}.
    The LLAVA Instruct 150k dataset is designed to enhance the training of multimodal models that interpret and respond to visual and textual instructions, featuring 150,000 instruction-response pairs derived from image-text pairs from public datasets like COCO and LAION. Utilizing GPT-4, these pairs are transformed into instruction-based queries that require understanding and reasoning about visual content, aligning responses with both direct descriptions and deeper inferential reasoning.

    \item \href{https://github.com/Vision-CAIR/MiniGPT-4}{\textbf{MiniGPT-4-IT}}~\cite{zhu2023minigpt4}.
    The MiniGPT-4-IT dataset is composed of 3,500 detailed image description pairs. These pairs were derived from a blend of sources including the Conceptual Captions, SBU, and LAION datasets. This collection was designed to train the MiniGPT-4 model to improve its language generation in response to visual inputs. The primary objective of the dataset is to facilitate the alignment of complex visual features with advanced language model capabilities, thereby enhancing the model's ability to generate natural and contextually appropriate descriptions for multimodal tasks. Essentially, MiniGPT-4-IT serves as a critical resource for bridging the gap between visual understanding and linguistic expression, aiming to boost the performance of AI models in interpreting and describing visual content.

    \item \href{https://github.com/Vision-CAIR/MiniGPT-4/blob/main/dataset/README_MINIGPTv2_FINETUNE.md}{\textbf{MiniGPT-v2-IT}}~\cite{chen2023minigptv2}.
    The MiniGPTv2-IT dataset, crafted for instruction tuning, integrates a variety of data types such as weakly-labeled image-text pairs, grounded captions, and fine-grained visual question answering (VQA) data across three training stages. Initial stages build broad vision-language capabilities using diverse sources like GRIT-20M, LAION, CC3M, and SBU. Later stages focus on fine-tuning with high-quality, task-specific datasets including COCO caption and RefCOCO. This structured approach enhances the model's efficiency in processing complex multimodal instructions and boosts its performance across various vision-language tasks. MiniGPTv2's training leverages millions of data points to develop robust multimodal interaction capabilities, making it a powerful tool in vision-language applications.

    \item \href{https://github.com/shikras/shikra}{\textbf{Shikra-IT}}~\cite{chen2023shikra}.
    The Shikra-IT dataset for instruction tuning includes two primary types of data: reorganized public datasets and newly generated high-quality RD data from Flickr30K Entities. It incorporates diverse sources such as VQA, Image Captioning datasets, and those with positional annotations like RefCOCO and Visual Genome. Additionally, 5,922 QA pairs were created using GPT-4, explicitly designed to include coordinate information in both questions and answers. This approach enhances the Shikra model's referential dialogue capabilities, enabling precise multimodal interactions. These interactions are crucial for applications that require accurate spatial references, such as augmented reality interfaces and visual customer support systems, where identifying and discussing specific areas within images are essential. The dataset effectively combines existing resources with AI-generated enhancements to train the model in handling complex, context-rich dialogues.

    \item \href{https://huggingface.co/datasets/THUDM/CogVLM-SFT-311K}{\textbf{CogVLM-SFT-311K}}~\cite{wang2024cogvlm}.
    The CogVLM-IT dataset integrates data from visual question-answering sources like VQAv2, OKVQA, TextVQA, and OCRVQA, along with dialogue datasets such as LLaVA-Instruct and LRV-Instruction, into a unified instruction-supervised fine-tuning framework. This collection trains the CogVLM model to enhance its multimodal interaction capabilities, enabling it to handle concise responses and detailed reasoning effectively. The dataset is crucial for ensuring the model’s robust performance across diverse visual and language tasks, significantly aiding in real-world applications that require precise and context-aware multimodal responses. This strategic compilation of varied data sources ensures comprehensive training and adaptability of the CogVLM model.

    \item \href{https://github.com/Efficient-Large-Model/VILA/tree/main/data_prepare}{\textbf{VILA-IT}}~\cite{lin2023vila}.
    The VILA-IT dataset is designed for instruction tuning with visual language models, blending 1 million text-only instruction data from FLAN with visual language datasets. This integration aims to address the degradation in text-only task performance while enhancing visual language capabilities. The dataset primarily includes visual question answering and caption style data, collected and generated to support joint supervised fine-tuning. This method significantly improves both text-based and visual task accuracies, demonstrating the effectiveness of merging text and visual data for training advanced visual language models. Overall, VILA-IT plays a crucial role in refining the performance of visual language models across diverse tasks.

    \item \href{https://huggingface.co/datasets/Lin-Chen/ShareGPT4V/tree/main}{\textbf{ShareGPT4V}}~\cite{chen2023sharegpt4v}.
    The ShareGPT4V dataset comprises 1.2 million detailed captions, initially created from 100K high-quality examples generated by GPT4-Vision. These captions were expanded using a specialized model to enhance multimodal model training, focusing on Supervised Fine-Tuning (SFT) and pre-training stages. The dataset emphasizes comprehensive coverage of topics such as world knowledge, object properties, and spatial relationships to improve modality alignment between visual and textual data. Utilized to develop the ShareGPT4V-7B model, it has shown superior performance across various benchmarks, demonstrating the benefits of detailed image-text pairs in multimodal interactions. ShareGPT4V exemplifies how rich, detailed captions can significantly boost the capabilities of large multimodal models.

    \item \href{https://huggingface.co/datasets/MBZUAI/GranD-f/tree/main}{\textbf{GranD}}~\cite{rasheed2023glamm}.
    The GranD dataset is a large-scale dataset containing 11 million images and 810 million regions with segmentation masks, created for training and evaluating models on visually grounded conversation tasks. This dataset is generated using an automated annotation pipeline that involves multi-level hierarchical structuring and state-of-the-art models to provide detailed object localization, attributes, and relationships. The dataset enables instruction-response pairs by using complex visual scenes structured as queries to generate contextually rich, detailed responses, intertwined with visual prompts that ensure accurate grounding in visual elements. GranD supports the Grounded Conversation Generation (GCG) task, producing responses integrating descriptions with segmentation masks. This focus on dense annotations and complex visual reasoning sets a new benchmark in multimodal datasets, advancing visually grounded language models.
    
    \item \href{https://github.com/RUCAIBox/ComVint/tree/main/ComVint/dataprocess}{\textbf{ComVint}}~\cite{du2023makes}.
    The ComVint dataset consists of 32K synthetic visual reasoning instructions designed to enhance the performance of multimodal large language models (MLLMs). Developed through a systematic multi-stage process of synthesis, complication, and reformulation, the dataset utilizes complex visual reasoning tasks to create instructions. The generation process starts with GPT-4 synthesizing an initial instruction from an image's annotations. Then, through an iterative "complicate-then-verify" paradigm, the complexity of these instructions is gradually increased, ensuring both the complexity and quality are maintained. The dataset primarily aims to boost MLLMs' capabilities in complex visual reasoning, demonstrating substantial improvements in model performance on comprehensive benchmarks. Overall, ComVint significantly contributes to advancing AI's ability to interpret and reason about complex visual inputs within a multimodal context.

    \item \href{https://arxiv.org/abs/2308.16463}{\textbf{SparklesDialogue}}~\cite{huang2023sparkles}.
    The SparklesDialogue dataset is crafted using a GPT-4 assisted process, where GPT-4 simulates realistic dialogues between a user and an assistant, involving multiple images. It is part of the Sparkles project, aimed at enhancing multimodal instruction-following models. Images and textual data are sourced from various image-caption pairs. During its construction, GPT-4 uses detailed image descriptions to generate dialogues, ensuring rich textual interaction while no actual images are sent to GPT-4. This process includes Dialogue Demonstrations, which serve as learning examples for creating coherent and contextually relevant dialogues, and Candidate Image Descriptions, which provide a diverse pool of images for generating discussions. This setup aids in training models like SparklesChat, enhancing their ability to handle intricate multimodal interactions. SparklesDialogue thus plays a crucial role in advancing complex managing, context-aware multimodal conversations and improving multimodal understanding capabilities.

    \item \href{https://github.com/SihengLi99/TextBind}{\textbf{TextBind}}~\cite{li2023textbind}.
    The TEXTBIND dataset from GPT-4 consists of 25,629 multi-turn conversations, integrating images and text to train models on multimodal instruction-response tasks. This dataset leverages a three-step pipeline involving topic-aware image sampling, LLM-generated dialogues, and rigorous post-processing. It sources images and text from publicly available image-caption pairs, designed to enhance language models' ability to handle complex, interleaved image-text content. TEXTBIND's primary feature is its focus on generating practical, context-rich conversations that reflect diverse real-world scenarios, supporting multimodal outputs. This approach significantly advances the capability of models to navigate open-ended, multimodal interactions, providing a robust platform for developing advanced generative models.

    \item \href{https://huggingface.co/datasets/PVIT/pvit_data_stage2/tree/main}{\textbf{PVIT}}~\cite{chen2023position}.
    The PVIT dataset consists of region-level instruction data, including 234k image-text pairs. This dataset is generated using three main strategies: 1) Dataset Conversion, where existing Visual Question Answering (VQA) datasets like GQA and VCR are reformatted into region-level instructions using specific templates, producing 146k entries. 2) Task-Specific Instruction Data Generation, which employs ChatGPT to create instructions for predefined multimodal tasks (e.g., object recognition), resulting in 20k single-turn and 66k multi-turn data entries, using detailed image annotations from datasets like MS COCO and Visual Genome. 3) General Instruction Data Generation improves diversity and quality by generating 22k entries with detailed descriptions and visual grounding annotations. These strategies collaboratively enhance the dataset's utility in training AI models for complex image-based instruction following, improving AI’s understanding and generation capabilities in diverse scenarios.

    \item \href{https://opendatalab.com/OpenDataLab/DataEngine-InstData}{\textbf{DataEngine-InstData}}~\cite{zhao2023mllm}. The DataEngine-InstData dataset is designed to enhance the instruction-following capabilities of AI models using a semi-automated process known as Interactive Prompt Optimization (IPO). This dataset contains QA pairs that are specifically generated using GPT-4, optimized through human collaboration to correct and refine prompts based on identified failures in preliminary tests. These corrections are focused on adhering to the desired question types and accurate use of bounding box annotations to reduce illusions. The process of creating these QA pairs includes manually designing initial prompts, testing, and refining based on failure analysis. The dataset serves to train AI in handling complex queries effectively, particularly improving performance on spatial and imaginative questions. The final dataset aims to provide robust training material that supports advanced AI learning protocols without incorporating inaccurate or inappropriate data.

\end{itemize}

\subsubsection{Video Instruction Tuning Datasets}\label{sec:appen:it:video}
In this subsubsection, we provide a comprehensive summary of video instruction tuning datasets to help people find the most suitable datasets for video instruction tuning.
\begin{itemize}
    \item \href{https://github.com/OpenGVLab/InternVideo/tree/main/Data/instruction_data}{\textbf{Video-Chat-Instruction}}~\cite{li2023videochat}. This multimodal instruction dataset was created using WebVid-10M as the foundation. This dataset includes 7,000 detailed video descriptions and 4,000 video-based conversations. The detailed descriptions and the multi-turn conversation generations were created by ChatGPT, which utilized the text from VideoChat-Text and several prompts focusing on the spatiotemporal aspects of the videos. To enhance the diversity of the video instruction data, video conversations were introduced, enriching the dataset with temporal and causal dynamics. This enriched dataset was employed to train models such as Videochat~\cite{li2023videochat} and Videollama~\cite{zhang2023video}.

    \item \href{https://github.com/OpenGVLab/Ask-Anything/tree/main/video_chat2}{\textbf{Video-Chat-Instruction}}~\cite{li2023mvbench}. The MVBench Instruction Tuning dataset comprises 1.9 million samples drawn from 34 diverse datasets across 6 categories. It was constructed by incorporating both image and video data in the instruction set to improve training for Multi-modal Large Language Models (MLLMs). This dataset can be used to address the limited diversity in instruction-tuning data and to evaluate the general capability of MLLMs for open-world temporal understanding, covering tasks from percwption to cognition. This enriched dataset was employed to train models such as Videochat2~\cite{li2023mvbench} and InternVideo2~\cite{wang2024internvideo2}.
\end{itemize}

\subsubsection{Audio Instruction Tuning Datasets}\label{sec:appen:it:audio}
\begin{itemize}
    \item \href{https://github.com/QwenLM/Qwen-Audio}{\textbf{Qwen-Instruction}}~\cite{chu2023qwen}.
    The Qwen-Audio Instruction Tuning dataset consists of 20k data points and is constructed by combining audio-centric instruction data with pure text instruction data. This dataset is designed to facilitate versatile input from both audio and text modalities within multi-turn dialogues. By leveraging this dataset during training, the model can seamlessly handle diverse forms of input, enabling effective interaction following human instructions.
    
    \item \href{https://audiodialogues.github.io/}{\textbf{Audio-Dialogues Instruction}}~\cite{goel2024audio}. 
    The Audio-Dialogues Instruction Tuning dataset comprises 163.8k samples and is designed to address the limitations of existing datasets by focusing on multi-turn dialogues for general sounds and music understanding. The dataset was constructed using a prompting-based approach with caption annotations from the AudioSet strongly labeled dataset and the MusicCaps dataset, guided by the GPT-4 model. This dataset aims to facilitate the training and evaluation of existing audio-augmented large language models on complex interactions regarding audio content, providing a valuable resource for tasks such as audio captioning, sound event classification, and music recommendation systems.

    \item \href{https://github.com/facebookresearch/fairseq/tree/main/examples/hubert}{\textbf{HuBERT Instruction}}~\cite{hsu2021hubert}. The HuBERT tokens Instruction Tuning dataset in the article consists of a substantial amount of data that is used for fine-tuning the model. This dataset is constructed by extracting tokens from audio instructions, providing a valuable resource for training the model to better understand and process spoken instructions. By leveraging this dataset, HuBERT can improve its performance in tasks related to processing and interpreting audio instructions, ultimately enhancing its ability to handle speech-based tasks effectively.

    \item \href{https://huggingface.co/datasets/LinkSoul/LLaSM-Audio-Instructions}{\textbf{LLaSM Instruction}}~\cite{shu2023llasm}. The LLaSM Instruction Tuning dataset, named LLaSM-Audio-Instructions, consists of a total of 199k conversation data and 508k samples. This dataset was constructed by generating audio data from language-only datasets and filtering out irrelevant conversations and chatbot responses. By utilizing Microsoft Azure text-to-speech API to convert human responses into speech data, the dataset provides complex instructions for fine-tuning the model. This dataset aims to address the scarcity of cross-modal speech-and-language instruction data and enhance the model's ability to follow multi-modal instructions effectively.

    \item \href{https://github.com/magic-research/bubogpt/blob/main/dataset/README.md#audio-dataset-instruction}{\textbf{BuboGPT-IT}}~\cite{zhao2023bubogpt}.
    The BuboGPT-IT dataset consists of three categories for instruction tuning. The image-text portion merges 3,439 pairs from MiniGPT-4 with 158K from LLaVA, focusing on detailed descriptions and complex reasoning. The audio-text dataset, termed Clotho-Detail, contains 3,938 extended audio captions, enhancing descriptive richness. The audio-image-text set, sourced from VGGSS, includes 5,158 triple-modality pairs, aligning sounds with their visual sources and incorporating negative pairs to improve semantic reasoning. These datasets were developed by augmenting existing data with AI-generated content, aiming to support complex multimodal interactions. They equip BuboGPT with the capability to handle sophisticated instruction-based tasks across various modalities, boosting its performance in intricate multimodal environments.
\end{itemize}

\subsubsection{3D Instruction Tuning Dataset}\label{sec:appen:it:3d}

\begin{itemize}
    \item \href{https://artemisp.github.io/X-InstructBLIP-page/}{\textbf{X-InstructBLIP}}~\cite{panagopoulou2023x}.
    The X-InstructBLIP's IT dataset is designed to support instruction tuning across multiple modalities including images, audio, video, and 3D models. It includes instruction-response pairs with 24K QA samples for audio and 250K QA samples for 3D. The data is collected by leveraging open-source large language models to generate question-answer pairs from existing captioning datasets, such as Cap3D for 3D models and AudioCaps for audio data. The dataset incorporates individual modality training to form cross-modal reasoning capabilities without extensive modality-specific pre-training. The primary feature of this dataset is its ability to facilitate the fine-tuning of instruction-modality alignment in a scalable and efficient manner, showcasing strong cross-modal reasoning by discerning between different modalities. In summary, the X-InstructBLIP's IT dataset exemplifies a comprehensive and scalable approach to instruction tuning, effectively handling diverse modalities and enhancing cross-modal reasoning tasks.

    \item \href{https://openlamm.github.io/}{\textbf{LAMM}}~\cite{yin2024lamm}.
    The LAMM dataset facilitates instruction-response pair training, containing 186,098 image-text pairs and 10,262 3D-text pairs from diverse publicly available datasets. Using the GPT-API, instructions and responses are generated through self-instruction methods based on the original dataset labels. This process involves extensive pre-processing, including the enrichment of visual information and conversion of vision task annotations into more comprehensible formats for MLLMs. LAMM uniquely emphasizes fine-grained information, supports commonsense knowledge through a hierarchical knowledge system, and enhances the understanding of vision-related instructions. It represents a significant stride in bridging modalities for AI training, leveraging detailed instructions to improve multimodal language model responsiveness and adaptability.
\end{itemize}

%%%%%%%%%%%%%%%%%%%%%%%%%%%%%

\subsection{Commonly Used MLLM Evaluation Benchmarks}\label{sec:appen:bench}
Given the abundance of research papers on image multimodality, we will separately discuss the evaluation datasets of image multimodality and the evaluation of other forms of multimodality.

\subsubsection{Image Data Multimodal Evaluation}\label{sec:appen:bench:image}
In this subsubsection, we summarize commonly used evaluation datasets that are utilized to assess the performance of image-text multimodal large language models (LLMs).

\paragraph{Image Caption and General VQA Evaluation Datasets.}Image captioning and general visual question answering (VQA) datasets serve as benchmarks for evaluating a model's comprehensive understanding of visual content. These datasets can also be utilized to assess the few-shot learning capabilities of multimodal large language models (LLMs) in the context of vision-language tasks, providing insights into their ability to generalize and adapt to new scenarios with limited training examples.
\begin{itemize}
    \item \href{https://mmmu-benchmark.github.io}{\textbf{MMMU}}~\cite{yue2023mmmu}.
    MMMU is a comprehensive multimodal benchmark that assesses models on their proficiency in college-level reasoning across multiple disciplines. Featuring 11,500 questions paired with complex images and text sourced from college exams, quizzes, and textbooks, it spans six core areas: Art \& Design, Business, Science, Health \& Medicine, Humanities \& Social Science, and Tech \& Engineering. The dataset challenges models with college-level tasks that require deep domain knowledge and sophisticated reasoning, closely mimicking the cognitive challenges faced by professionals. MMMU's detailed creation process ensures the accuracy and relevance of its content, testing models on perception, knowledge comprehension, and logical reasoning. This dataset is pivotal for advancing model capabilities in handling intricate, multimodal data in specialized academic fields.

    \item \href{https://arxiv.org/abs/2306.13394}{\textbf{MME}}~\cite{fu2024mme}.
    The MME dataset, structured into MMEP (Perception) and MMEC (Cognition) components, is designed for evaluating multimodal large language models. It comprises 14 sub-tasks across both segments, focusing on object recognition, optical character recognition, and advanced reasoning tasks like commonsense reasoning and numerical calculations. The dataset features image-text pairs and instructions, all manually created to avoid data leakage by excluding public dataset dependencies. Images are sourced from real photographs and other collections, tailored to test both basic and advanced multimodal understanding. MME challenges models to respond to concise, human-like prompts, pushing their capabilities in visual comprehension and cognitive processing. This benchmark is a comprehensive tool for revealing and enhancing the abilities of multimodal models, emphasizing their performance in complex, real-world tasks that blend visual perception with cognitive operations.

    % \item \href{https://shannon.cs.illinois.edu/DenotationGraph/}{\textbf{Flickr30K}}~\cite{young2014image} image-text retrieval benchmarks
    
    % \item \href{https://cocodataset.org/#home}{\textbf{MS-COCO}} benchmark

    \item \href{https://github.com/nocaps-org}{\textbf{Nocaps}}~\cite{agrawal2019nocaps}. The Nocaps dataset features images from the Open Images V4~\cite{kuznetsova2020open} validation and test sets, carefully selecting images to diversify object representation and avoid bias towards common classes like person, car, or plant. This selection aims to address the gap in COCO Captions~\cite{chen2015microsoft}, where nearly 400 out of 500 specific classes (excluding overly broad or infrequent ones) are seldom mentioned. Captions for nocaps, including human-generated baselines, were gathered through a specially adapted COCO collection interface, emphasizing high-quality contributions by employing only US-based Amazon Mechanical Turk workers with over 5,000 tasks and a 95\% approval rate. A total of 727 workers contributed, averaging 228 captions each, resulting in a comprehensive set of 166,100 nocaps captions.

    \item \href{https://cs.stanford.edu/people/dorarad/gqa/about.html}{\textbf{GQA}}~\cite{hudson2019gqa}.
    Current VQA benchmarks fail to provide accurate indication of visual understanding capacity. Not only are they severely biased, they also lack semantic compositionality, and do not provide any tools or measures to gain significant insight into models' performance and behavior.
    The authors design a new dataset, GQA, to address these shortcomings, featuring compositional questions over real-world images. The dataset consists of 22M questions over 113K various day-to-day images. 
    To construct the GQA dataset, a wide array of real-world images depicting everyday scenes was selected from sources like Visual Genome. For each chosen image, detailed scene graphs were generated, describing the objects present, their attributes, and the relationships among them, utilizing advanced computer vision techniques. Questions probing both the direct content of the images and requiring deeper reasoning about the scenes were then crafted based on these graphs. Each question was provided with a structured semantic representation—a functional program that outlines the logical steps necessary for answering it. Throughout the creation process, the data underwent rigorous cleaning and validation to ensure accuracy and consistency across images, scene graphs, questions, and their semantic frameworks. Many of the GQA questions involve multiple reasoning skills, spatial understanding and multi-step inference, thus are generally more challenging than previous visual question answering datasets used in the community. 

    \item \href{https://github.com/kushalkafle/DVQA_dataset}{\textbf{DVQA}}~\cite{kafle2018dvqa}.
    The DVQA dataset is designed to evaluate the comprehension of bar charts through a question-answearing framework, aiming to enhance algorithms' ability to extract and interpret numeric and semantic information from a variety of bar chart styles found in diverse sources like scientific publications and business reports. Comprising over 3 million image-question pairs, DVQA emphasizes not just basic visual recognition but also complex cognitive tasks such as pattern matching, attention, and reasoning. It challenges existing visual question answering models with unique demands, such as handling dynamically generated text and answers specific to each chart, thus pushing forward the capability of AI systems to interact with and understand structured visual data effectively.

    \item \href{https://github.com/cambridgeltl/visual-spatial-reasoning?tab=readme-ov-file}{\textbf{VSR}}~\cite{liu2023visual}.
    Visual Spatial Reasoning (VSR) is a dataset comprising over 10,000 natural text-image pairs with 66 types of spatial relations in English, such as under, in front of, and facing. The dataset aims to highlight the challenges in capturing relational information for current vision-and-language models. Research indicates a significant performance gap between humans (achieving above 95\% accuracy) and state-of-the-art models (reaching around 70\% accuracy) on spatial reasoning tasks. VSR emphasizes the difficulties that current models face in recognizing spatial relations concerning object orientations and notes their poor generalization on unseen concepts. Through comprehensive analysis on popular vision-language models, it underscores the importance of positional encodings, the lack of correlation between model performance and training examples, and the specific challenges posed by certain spatial relations. The findings from VSR provide a realistic evaluation of models' performance in understanding spatial relations.

    \item \href{https://okvqa.allenai.org/}{\textbf{OKVQA}}~\cite{marino2019ok}.
    The OK-VQA dataset was created to address the limitations of existing VQA benchmarks by focusing on knowledge-based visual question answering. This dataset consists of over 14,000 questions that require external knowledge to answer, covering various categories such as science \& technology, history, and sports. The questions in OK-VQA challenge models to not only understand the image and question but also to retrieve and incorporate relevant knowledge from external sources. By providing a diverse and difficult set of questions, the OK-VQA dataset enables researchers to evaluate the reasoning capabilities of VQA models in scenarios where answers cannot be obtained solely from the image. This dataset opens up new research opportunities in the domain of knowledge-based visual question answering.

    \item \href{https://vizwiz.org/}{\textbf{Vizwiz}}~\cite{gurari2018vizwiz}.
    The VizWiz dataset was created by collecting visual questions from blind individuals seeking answers to daily visual challenges. This dataset stands out from others as it includes images taken by blind photographers, presenting challenges like image blur and poor lighting. The questions in VizWiz are spoken, reflecting a more conversational style and potential audio recording imperfections. By addressing real-world interests of blind users, the dataset aims to empower them in overcoming visual-based obstacles. Modern algorithms face difficulties in answering questions from VizWiz due to its unique characteristics, highlighting the need for specialized solutions to assist blind individuals effectively.

    \item \href{https://github.com/RUCAIBox/POPE}{\textbf{POPE}}~\cite{li2023evaluating}
    The "POPE" dataset focuses on evaluating object hallucination in vision-language models, using 6,136 binary questions to test if models hallucinate non-existent objects in images from MSCOCO and other sources. Each image is analyzed to establish a ground truth for yes-or-no queries about specific objects, ensuring each question corresponds accurately to image content. POPE assesses the reliability and accuracy of models in interpreting visual data by highlighting their propensity to generate hallucinatory content. This benchmark is crucial for testing object recognition accuracy and addressing significant challenges in model reliability for practical real-world applications.
\end{itemize}

\paragraph{Text-Oriented VQA Evaluation Datasets} While image captioning and general VQA datasets primarily focus on evaluating an algorithm's understanding of visual content, some datasets in these categories also include questions that require reading and comprehending text present in the images, thus providing a test for the text recognition capabilities of the models.

\begin{itemize}
    \item \href{https://textvqa.org/}{\textbf{TextVQA}}~\cite{singh2019towards}.
    The TextVQA dataset was created by selecting images containing text from the Open Images dataset through a three-stage crowdsourcing process, resulting in 28,408 images forming the basis of the dataset. Each image had 1-2 questions collected, with the first question requiring reading the text in the image to answer and the second question requiring reasoning about the text for a different answer. The dataset's characteristics include a focus on text-related questions that require reading and reasoning about text in images, encouraging research on improving text detection and recognition in unconstrained environments, and enabling VQA models to read and reason about text in images. The dataset also introduces the LoRRA model architecture, which reads text in images, reasons about it based on the question, and predicts answers from a fixed vocabulary or the text found in the image. This dataset and model facilitate exploration and solutions for questions involving text in images in the VQA domain.

    \item \href{https://www.docvqa.org/}{\textbf{DocVQA}}~\cite{mathew2021docvqa}.
    The DocVQA dataset was created by collecting document images from the UCSF Industry Documents Library, spanning various industries and document types. The dataset consists of 50,000 questions on 12,000+ document images, with questions and answers collected through a web-based annotation tool. The dataset stands out for its focus on VQA on document images, requiring models to interpret text within the layout and structure of the documents. This dataset addresses the challenge of extracting information from document images through natural language questions, encouraging models to understand textual, graphical, and structural elements in the documents. It serves as a valuable resource for developing and evaluating models that can effectively answer questions based on the content of document images.

    \item \href{https://github.com/vis-nlp/ChartQA}{\textbf{ChartQA}}~\cite{masry2022chartqa}.
    The ChartQA dataset was created by generating human-authored question-answer pairs based on real-world charts, aiming to address the limitations of existing datasets that rely on template-based questions and automatically generated charts. This dataset stands out for its diverse question types involving visual and logical reasoning, allowing for more complex analysis of chart data. By combining visual features and extracted data tables from chart images, the dataset enables the development of transformer-based QA models that achieve state-of-the-art results in handling questions that require both visual and logical reasoning.

    \item \href{https://allenai.org/data/diagrams}{\textbf{AI2D}}~\cite{kembhavi2016diagram}.
    The AI2D dataset was created by compiling over 5000 grade school science diagrams with more than 150,000 rich annotations, including ground truth syntactic parses and over 15,000 multiple choice questions. The diagrams were collected by scraping Google Image Search using seed terms from science textbooks. Each image was annotated using Amazon Mechanical Turk in a multi-phase process to ensure high agreement levels among annotators. The dataset's rich annotations categorize constituents, relationships, and textual elements within the diagrams, making it a valuable resource for tasks such as syntactic parsing, semantic interpretation, and diagram question answering. The AI2D dataset's unique characteristics and comprehensive annotations provide a solid foundation for advancing research in diagram interpretation and reasoning.

    \item \href{https://ocr-vqa.github.io/}{\textbf{OCR-VQA}}~\cite{mishra2019ocr}.
    The OCR-VQA dataset creation process involved obtaining book cover images with metadata, generating question-answer pairs, and annotating the dataset. This dataset stands out for its focus on visual question answering by reading text in images, filling a gap in traditional VQA literature. It addresses challenges such as robust layout analysis, OCR for fancy fonts, and identifying book categories based on covers. The dataset's unique characteristics enable researchers to explore new avenues in document image analysis and VQA, offering a valuable resource for studying text-based visual question answering tasks.

    \item \href{https://scienceqa.github.io/}{\textbf{ScienceQA}}~\cite{lu2022learn}
    The "Science QA" evaluation dataset, sourced from IXL Learning, features approximately 21,000 multimodal questions from science curricula, aimed at testing AI's multi-hop reasoning abilities. Each question is accompanied by images and detailed explanations, also from IXL Learning, designed to mimic educational standards and reasoning processes. This dataset significantly preprocesses content to ensure relevance and educational alignment, evaluating AI's capability to integrate multimodal inputs and external knowledge into coherent answers. "Science QA" serves as a benchmark for AI models, emphasizing their interpretability and reliability in reasoning within educational contexts. It challenges AI systems to not only provide answers but also generate understandable explanations, pushing forward the development of AI technologies that can effectively support educational applications

    \item \href{https://mathvista.github.io/}{\textbf{MathV}}~\cite{lu2023mathvista}
    The "MathV" dataset comprises 6,141 image-text pairs from 31 multimodal datasets, including 28 existing and three new ones (IQTest, FunctionQA, PaperQA). Images are sourced from diverse contexts such as natural scenes and scientific diagrams. Questions and answers, rooted in various mathematical reasoning types (algebraic, arithmetic, statistical), are generated from these visuals. The dataset is meticulously annotated with metadata to categorize each example by task type, grade level, and required reasoning skills. "MathV" primarily serves as a comprehensive benchmark for evaluating the mathematical reasoning capabilities of AI models in visual contexts. It aims to assess and advance the development of AI models, particularly foundation models, by challenging their ability to interpret and solve visually-based mathematical problems, revealing both their strengths and limitations in real-world applications.

    \item \href{https://github.com/yuweihao/MM-Vet}{\textbf{MMVet}}~\cite{yu2023mmvet}
    The "MMVet" dataset is a benchmark for evaluating large multimodal models (LMMs) on complex tasks. It includes 200 images and 218 questions that span six core capabilities: recognition, OCR, knowledge, language generation, spatial awareness, and math. These components are integrated to assess the models' ability to handle real-world scenarios effectively, such as interpreting jokes or solving visual arithmetic problems. Questions and images are sourced from diverse online platforms, including specialized domains like medical imaging. MMVet employs an LLM-based evaluator, notably using models like GPT-4, to score responses based on their conformity to varied answer styles and question types, adapting to the multifaceted nature of real-world applications. This benchmark challenges models to synthesize and apply multiple capabilities, providing a realistic assessment of their practical utility.
\end{itemize}

\paragraph{Refer Expression Comprehension Evaluation Datasets.} Referring Expression Comprehension (REC) evaluation datasets, such as RefCOCO, RefCOCO+, and RefCOCOg, are essential for assessing models' ability to understand and ground natural language expressions in visual contexts. These datasets consist of images paired with referring expressions that describe specific objects or regions. The task involves accurately identifying the referred object based on the given expression. REC datasets challenge models to bridge the gap between vision and language, requiring the capture of fine-grained details, spatial relationships, and contextual information. They serve as benchmarks for evaluating the performance of models in understanding referring expressions, contributing to advancements in vision-language integration with various applications.

\begin{itemize}
    \item \href{https://github.com/lichengunc/refer}{\textbf{RefCOCO, RefCOCO+, RefCOCOg}}~\cite{kazemzadeh2014referitgame, mao2016generation}.
    The RefCOCO dataset, built upon the MS COCO dataset, consists of 142,209 referring expressions corresponding to 50,000 objects in natural images. The referring expressions in RefCOCO are generated with a focus on the target objects, providing a dataset suitable for studying object-centric referring expression comprehension. The dataset includes segmentation masks for the target objects, enabling pixel-level analysis and evaluation. RefCOCO serves as a valuable resource for developing and benchmarking algorithms that aim to accurately ground referring expressions to specific objects within an image.
    
    RefCOCO+ is an extension of the RefCOCO dataset, also utilizing images from MS COCO. It contains 141,564 referring expressions, corresponding to 49,856 objects. The key difference between RefCOCO and RefCOCO+ lies in the way the referring expressions are generated. In RefCOCO+, the expressions are collected with a focus on the entire image context, resulting in expressions that may include more background information and irrelevant details. This dataset challenges algorithms to handle referring expressions that are not solely centered around the target objects, requiring a deeper understanding of the image context. Like RefCOCO, RefCOCO+ provides segmentation masks for the target objects.
    
    RefCOCOg sets itself apart from RefCOCO and RefCOCO+ by utilizing images sourced from Google search results. It consists of 95,010 referring expressions, corresponding to 49,822 objects. The referring expressions in RefCOCOg are collected independently of the images, resulting in more natural and diverse expressions. Unlike the other two datasets, RefCOCOg includes both object categories and stuff categories, such as "sky" and "grass," expanding the scope of referring expression comprehension. However, RefCOCOg only provides bounding box annotations for the target objects and does not include pixel-level segmentation masks.
    
    These three datasets offer distinct challenges and opportunities for researchers working on referring expression comprehension. 

    \item \href{https://allenai.org/project/grit/home}{\textbf{GRIT}}~\cite{gupta2022grit}.
    The GRIT dataset was meticulously designed with specific principles in mind to address key challenges in computer vision research. The dataset creation process focused on selecting unambiguous tasks with clear definitions and unambiguous ground truth, similar to the approach taken in the GLUE benchmark. By including a variety of tasks such as object categorization, object localization, referring expressions, visual question answering, semantic segmentation, human keypoint estimation, and surface normal estimation, GRIT covers a broad range of visual skills. One of the unique features of GRIT is its evaluation of generalization to new data sources and concepts, robustness to image perturbations, and calibration measures, which are crucial for developing more flexible and general computer vision systems. Additionally, GRIT offers two tracks, Restricted and Unrestricted, to support the development of large-scale models and fair comparisons between models with varying compute resources. Overall, the GRIT dataset serves as a unified platform for assessing the overall capability of computer vision systems across diverse concepts and data sources, aiming to drive the development of performant and robust general-purpose vision systems.
\end{itemize}

\paragraph{Instruction Following Evaluation Datasets} Instruction Following Evaluation Datasets assess models' ability to understand and execute natural language instructions in various domains. These datasets consist of high-level instructions paired with corresponding actions, challenging models to interpret complex instructions, reason about necessary steps, and generate appropriate outputs. They advance research in natural language processing, robotics, and embodied AI, providing benchmarks for evaluating approaches and techniques. They contribute to developing intelligent agents that can assist humans, enhance productivity, and enable more natural human-machine interactions.

\begin{itemize}
    \item \href{https://allenai.org/project/grit/home}{\textbf{TouchStone}}~\cite{bai2023touchstone}.
    The TouchStone dataset creation process involved curating a diverse visual dialogue dataset encompassing five major categories of abilities and 27 subtasks. This dataset was carefully constructed to cover not only basic recognition and comprehension but also extend to literary creation and analysis abilities. One key feature of the TouchStone dataset is the integration of detailed image annotations, which enable the transformation of multimodal input content into a form understandable by advanced language models. This innovative approach allows for the direct evaluation of the quality of multimodal dialogue without the need for human intervention. By providing a comprehensive assessment of the capabilities of multimodal language models, the TouchStone dataset addresses the challenge of evaluating large vision-language models in open-ended dialogues, offering a standardized and objective method for assessing performance.

    \item \href{https://allenai.org/project/grit/home}{\textbf{SEED-Bench}}~\cite{li2023seed}.
    SEED-Bench dataset was meticulously curated through a multi-step process involving data collection, human annotation, and automated filtering mechanisms. This dataset stands out due to its comprehensive coverage of 12 evaluation dimensions, encompassing both spatial and temporal understanding in images and videos. By providing 19K multiple-choice questions with accurate annotations, SEED-Bench offers a robust platform for evaluating the generative comprehension capabilities of Multimodal Large Language Models (MLLMs). Researchers can leverage this dataset to address critical issues related to model performance, comprehension accuracy, and the effectiveness of generative models in processing multimodal inputs.

    \item \href{https://allenai.org/project/grit/home}{\textbf{MME}}~\cite{fu2024mme}.
    The MME dataset in the article was meticulously created through manual design of instruction-answer pairs to prevent data leakage and ensure fair comparison of MLLMs. The dataset features a total of 14 subtasks covering perception and cognition abilities, including tasks like text translation, code reasoning, and arithmetic problems. By providing concise instructions and utilizing real photographs for data collection, the MME dataset addresses the need for a comprehensive evaluation of MLLMs, highlighting areas for model improvement and guiding future development in the field.

    \item \href{https://github.com/haotian-liu/LLaVA}{\textbf{LLaVAW}}~\cite{liu2024visual}
    The "LLaVA-Bench (In-the-Wild)" dataset serves as an evaluation benchmark to test the capability of models on complex reasoning in diverse environments. It comprises 24 images with 60 questions, featuring a variety of visual content including indoor and outdoor scenes, memes, paintings, and sketches. Each image is paired with a detailed, manually-curated description and a set of carefully selected questions.  This benchmark focuses on evaluating the generalizability and adaptability of models to novel domains and their ability to handle complex reasoning across varied visual contexts.
\end{itemize}

\paragraph{Other MM Evaluation Datasets}Evaluation Datasets are not limited to the aforementioned aspects. Other datasets can provide a more comprehensive understanding of the capabilities of large models from various perspectives. 
\begin{itemize}
    \item \href{https://ai.meta.com/blog/hateful-memes-challenge-and-data-set/}{\textbf{HM}}~\cite{kiela2020hateful}.
    The Hateful Memes dataset was created as a challenge set to detect hate speech in multimodal memes. The dataset was carefully constructed to be challenging for unimodal architectures by including "benign confounders" that can flip the label of a hateful meme. It consists of examples with high-confidence ratings from trained annotators and is balanced to include various multimodal fusion problems. This dataset aims to address the societal problem of hate speech by requiring reasoning about subtle cues in memes. It provides insights into the distribution of protected categories, types of attacks, and lexical statistics, highlighting the need for improvements in machine learning systems to tackle hate speech effectively.

    \item \href{https://github.com/open-compass/MMBench}{\textbf{MMB}}~\cite{liu2023mmbench}
    The "MMBench" dataset is a comprehensive benchmark designed for evaluating large vision-language models (VLMs), consisting of around 3,000 single-choice questions that assess 20 distinct abilities ranging from object localization to social reasoning. Questions and choices are drawn from a mix of custom-generated and ChatGPT-assisted content, with images sourced from datasets like COCO-Caption and Places. MMBench utilizes a "Circular Evaluation" strategy, which tests models' robustness by rotating answer choices across multiple rounds. This method enhances the reliability of assessing models' perception, reasoning, and instruction-following abilities. MMBench aims to provide detailed insights into AI models' capabilities, addressing the limitations of traditional benchmarks by focusing on fine-grained skills and employing AI for precise answer matching, thereby advancing the field of AI by delineating the strengths and weaknesses of current multimodal models.
\end{itemize}

%%%%%%%%%%%%%%%%%%%%%%%
\subsubsection{Video Data Multimodal Evaluation}\label{sec:appen:bench:video}
In this subsubsection, we summarize commonly used evaluation datasets for video-text multimodal large language models (LLMs). Since many datasets are versatile enough to handle multiple evaluation tasks, our classification is provided for reference purposes only.

\paragraph{Video Question Answering}
Video question answering evaluation can evaluate the model's video understanding and question answering ability.
\begin{itemize}
    \item \textbf{MSVD}~\cite{chen2011collecting}. The MSVD dataset consists of 2,089 video segments and 85,550 English descriptions, with an average of 41 descriptions produced for each video, and at least 27 descriptions for over 95\% of the videos. Even when focusing on descriptions from Tier-2 tasks, there are still 16 descriptions on average for each video, with at least 12 descriptions for over 95\% of the videos. This dataset was constructed by asking annotators to watch short video clips and describe the main action or event in one sentence. The data collection framework used in this study involved deploying tasks on Amazon's Mechanical Turk platform, where video segments were selected from YouTube. The highly parallel nature of the data allows for the creation of monolingual parallel training data, which can be beneficial for tasks such as paraphrase evaluation.

    \item \textbf{MSR-VTT}~\cite{xu2016msr}. The MSR-VTT dataset is a significant contribution to the field of video understanding and language translation. It comprises 10K web video clips totaling 41.2 hours of content, with each clip annotated with about 20 natural sentences. The dataset was constructed by collecting 257 popular queries from a commercial video search engine, with 118 videos for each query, and annotating the clips with diverse and comprehensive categories. This large-scale dataset addresses the limitations of existing benchmarks by providing a wide variety of video content and associated language descriptions, enabling researchers to explore and develop more advanced algorithms for tasks such as video-to-text translation and video understanding.
    
    \item \textbf{TGIF-QA}~\cite{jang2017tgif}. The TGIF-QA dataset comprises 165,165 QA pairs extracted from 71,741 animated GIFs. The dataset was constructed by employing a combination of crowdsourcing and template-based approaches, generating questions based on video content. It introduces unique tasks for video VQA, such as counting repetitions of actions, identifying repeated actions, and recognizing state transitions in videos. These tasks require spatio-temporal reasoning and offer a new perspective on visual question answering in the video domain.

    \item \textbf{ActivityNet-QA}~\cite{yu2019activitynet}. The ActivityNet-QA dataset consists of 58,000 QA pairs derived from 5,800 complex web videos. The dataset was constructed by sampling videos from the larger ActivityNet dataset and generating QA pairs for each video. This dataset can be utilized to address challenges in VideoQA, enabling researchers to explore various video representation strategies and improve the performance of question answering systems for long web videos.

    \item \textbf{LSMDC}~\cite{rohrbach2017movie}. Large Scale Movie Description Challenge The LSMDC dataset consists of 118,114 sentences aligned with video clips from 202 movies. This dataset was constructed by collecting transcribed Audio Descriptions (ADs) and movie scripts, providing a rich source of visual and textual information for research purposes. Researchers can leverage this dataset to address challenges in generating video descriptions, understanding the relationship between visual content and language, and developing technologies to assist visually impaired individuals in accessing movie content.

    \item \textbf{MoVQA}~\cite{rohrbach2017movie}. The MoVQA dataset consists of 21,953 manually annotated question-answer pairs sourced from 100 movies of diverse genres. The dataset is designed to assess model capabilities in long-form video understanding across different temporal lengths, with questions categorized into six types: information synopsis, temporal perception, spatial perception, causal reasoning, hypothetical reasoning, and external knowledge. By segmenting movies into single-scene, multi-scene, and full-scene levels, MoVQA provides a comprehensive platform for integrating multimodal information and addressing complex cognitive challenges in movie comprehension.

\end{itemize}

\paragraph{Video Captioning and Video Retrieval}
Video captioning and video retrieval datasets serve as benchmarks for evaluating a model’s understanding of video content. 
\begin{itemize}
    \item \textbf{DiDeMo}~\cite{anne2017localizing}. The DiDeMo dataset consists of over 10,000 unedited personal videos with 3-5 pairs of descriptions and distinct moments per video. The dataset was constructed in two phases: first, annotators watched videos, selected moments, and described them to ensure another user could select the same moment based on the description. Second, collected descriptions were validated by annotators marking corresponding moments in the videos. This dataset addresses the challenge of localizing moments in video with natural language by providing pairs of localized video segments and referring expressions that uniquely identify specific moments in the videos.

    \item \textbf{VATEX}~\cite{wang2019vatex}. The VATEX dataset comprises over 41,250 videos paired with 825,000 captions in both English and Chinese, including more than 206,000 English-Chinese parallel translation pairs. The dataset was constructed by collecting English and Chinese descriptions for video clips from the Kinetics-600 validation and holdout test sets using Amazon Mechanical Turk. This dataset enables researchers to address various challenges in multilingual visual understanding, such as multilingual video captioning, enhancing video dynamics comprehension, and exploring the interaction between videos and multilingual knowledge. Additionally, the dataset supports tasks like visual question answering, natural language moment retrieval, and multilingual visual concept clustering, facilitating large-scale training for multilingual, multimodal research endeavors.
\end{itemize}

\paragraph{Other Video Evaluation Datasets}
Here, we summarize other evaluation datasets. Some are very comprehensive, while others offer unique video evaluations.
\begin{itemize}
    \item \href{https://github.com/OpenGVLab/Ask-Anything/tree/main/video_chat2}{\textbf{MVBench}}~\cite{li2023mvbench}. The MVBench dataset comprises 20 challenging video tasks that require both spatial and temporal understanding. It was constructed using a static-to-dynamic method, which adapts static image tasks with dynamic goals to systematically design temporal tasks for video comprehension. This dataset can be utilized to evaluate the comprehension capabilities of Multi-modal Large Language Models (MLLMs) in open-world temporal understanding, ranging from perception to cognition. It also includes 1.9 million diverse instructional data points, which can be utilized to enhance a model's ability to follow instructions.

    \item \href{https://egoschema.github.io/}{\textbf{EgoSchema}}~\cite{mangalam2024egoschema}. The EgoSchema dataset comprises over 5000 very long-form video language understanding questions derived from 250 hours of diverse egocentric video data. This dataset was manually curated to include questions that require choosing the correct answer from five choices based on a three-minute video clip, with a median certificate length of about 100 seconds. EgoSchema stands out from other video understanding datasets by featuring significantly longer temporal certificates, challenging state-of-the-art models that struggle in zero-shot evaluation scenarios. The dataset serves as a benchmark for evaluating and improving the capabilities of modern vision and language systems in comprehending complex and extended video content.
    
    \item \href{https://github.com/mbzuai-oryx/Video-ChatGPT/blob/main/quantitative_evaluation/README.md}{\textbf{VideoChatGPT}}~\cite{maaz2023video}. The dataset used for evaluating VideoChatGPT consists of 100,000 video-instruction pairs. This dataset was constructed through a combination of human-assisted annotation, where expert annotators provided detailed descriptions of video content, and semi-automatic annotation, which generated high-volume annotations using state-of-the-art vision-language models. The dataset is diverse and comprehensive, covering a wide range of data types such as detailed descriptions, question-answer pairs, and tasks stimulating creativity. This extensive dataset is crucial for training VideoChatGPT to comprehend video content effectively, integrating spatial and temporal cues into its understanding. It can be utilized to address challenges in video-based conversation models, such as improving temporal understanding, spatial consistency, and contextual comprehension.

    \item \href{https://github.com/jiyanggao/TALL}{\textbf{Charade-STA}}~\cite{gao2017tall}. The Charades-STA dataset consists of around 10,000 videos, each with temporal activity annotations from 157 activity categories and multiple video-level descriptions. To address the need for clip-level sentence annotations in Temporal Activity Localization via Language Query (TALL), the Charades-STA dataset was constructed by generating sentence temporal annotations for the original Charades dataset. This involved connecting consecutive sub-sentences within each video to create complex queries, ensuring the time span of each query was less than half of the video length. The dataset contains 13,898 clip-sentence pairs in the training set, 4,233 pairs in the test set, and 1,378 complex sentence queries. This dataset enables researchers to explore the potential of the CTRL framework in handling longer and more complex sentences for temporal activity localization tasks.

    \item \href{https://github.com/jayleicn/moment_detr/tree/main/data}{\textbf{QVHighlight}}~\cite{lei2021detecting}. The QVHIGHLIGHTS dataset consists of over 10,000 YouTube videos that cover a wide range of topics, such as everyday activities, travel, social and political events. Each video in the dataset is annotated with a human-written natural language query, relevant moments in the video corresponding to the query, and saliency scores for all query-relevant clips. This comprehensive annotation allows for the development and evaluation of systems that can detect relevant moments and salient highlights for diverse user queries. The dataset was constructed to address the challenge of the lack of annotated data for detecting moments and highlights in videos, providing a valuable resource for research in this area.
    
\end{itemize}

\subsubsection{Audio Evaluation Datasets}\label{sec:appen:bench:audio}
In this section, we give a comprehensive summary of commonly used evaluation datasets for audio-text multimodal large language models (LLMs).

\paragraph{Audio-Text Retrieval}
Audio retrieval datasets serve as benchmarks for evaluating a model’s understanding of audio content. 
\begin{itemize}
    \item \href{https://audiocaps.github.io/}{\textbf{AudioCaps}}~\cite{kim2019audiocaps}. The AudioCaps dataset consists of 46,000 pairs of audio clips and human-written text descriptions. This dataset was constructed by collecting data through crowdsourcing on the AudioSet dataset, ensuring that the captions are faithful to the audio inputs. The dataset can be utilized to address the task of audio captioning for sound in the wild, providing a valuable resource for developing and evaluating models that generate natural language descriptions for audio content.

    \item \href{https://zenodo.org/records/4743815}{\textbf{Clotho}}~\cite{drossos2020clotho}. The Clotho dataset for audio captioning consists of 4981 audio samples ranging from 15 to 30 seconds in duration and 24,905 captions with lengths between eight to 20 words. The dataset was constructed by collecting audio samples from the Freesound platform, processing them to meet specific criteria, and crowdsourcing captions using Amazon Mechanical Turk and annotators from English-speaking countries. Clotho aims to address the task of general audio content description through free text, providing a diverse set of audio samples and captions for research in audio captioning methods.
\end{itemize}

\paragraph{Audio Question Answering}
Audio question answering evaluation can evaluate the model's audio understanding and question answering ability.
\begin{itemize}
    \item \href{https://zenodo.org/records/6473207}{\textbf{ClothoAQA}}~\cite{lipping2022clotho}. The Clotho-AQA dataset consists of 1991 audio files, each lasting between 15 to 30 seconds, selected from the Clotho dataset. For each audio file, six different questions were collected through crowdsourcing using Amazon Mechanical Turk, with corresponding answers provided by different annotators. Two of the questions for each audio file are designed to have 'yes' or 'no' answers, while the remaining questions have single-word answers. This dataset was created to address the task of audio question answering, where a system analyzes both the audio signal and a natural language question to generate a relevant natural language answer.

    \item \href{https://gewu-lab.github.io/MUSIC-AVQA/}{\textbf{Audio-MusicAVQA}}~\cite{li2022learning}. The MUSIC-AVQA dataset in the article comprises over 45,000 question-answer pairs derived from more than 9,000 videos, totaling over 150 hours of content. The dataset was constructed by collecting real musical performance videos from YouTube, covering solo performances, ensembles of the same instrument, and ensembles of different instruments. The dataset includes 33 question templates across 9 question types, facilitating spatio-temporal reasoning over audio-visual scenes. Researchers can leverage this dataset to explore multimodal scene understanding, study audio-visual interactions, and advance spatio-temporal reasoning in dynamic audio-visual scenarios.
\end{itemize}
